# Supplementary material for: Accounting for not-at-random missingness through imputation stacking
Source: arXiv:2101.07954 ancillary file (2021-01-20)
Supplement: Supplementary file 1 [file Supplementary_Materials.pdf]

# Supplementary Materials for “Accounting for not-at-random missingness through imputation stacking” by

Lauren J. Beesley<sup>\*1</sup> and Jeremy Taylor<sup>1</sup>

<sup>1</sup>University of Michigan, Department of Biostatistics

<sup>\*</sup>Corresponding Author: lbeesley@umich.edu

## A An extension to multiple variable MNAR missingness

In this section, we provide a generalization of the proposed method that allows for MNAR missingness in *multiple* variables, with some restrictions. Suppose the columns of  $Z$  are ordered such that the first  $d$  variables are assumed to be MNAR. We make the following assumptions.

Suppose we partition the joint model for missingness as

$$f(\mathcal{R}_{i1}, \dots, \mathcal{R}_{ik} | Z_{i.}) = f(\mathcal{R}_{i,d+1}, \dots, \mathcal{R}_{ik} | Z_{i.}, \mathcal{R}_{i1}, \dots, \mathcal{R}_{id}) \\ \times f(\mathcal{R}_{id} | Z_{i.}, \mathcal{R}_{i1}, \dots, \mathcal{R}_{i,d-1}) \times \dots \times f(\mathcal{R}_{i2} | Z_{i.}, \mathcal{R}_{i1}) f(\mathcal{R}_{i1} | Z_{i.}).$$

where  $f$  denotes the distribution function for the corresponding variables. We will assume the following:

1.  $Z_{i,d+1}, \dots, Z_{ik}$  are MAR, with  $f(\mathcal{R}_{i,d+1}, \dots, \mathcal{R}_{ik} | Z_{i.}, \mathcal{R}_{i1}, \dots, \mathcal{R}_{id}) = f(\mathcal{R}_{i2}, \dots, \mathcal{R}_{ik} | W_{i.})$ .
2. For  $j = 1, \dots, d$ ,  $Z_{ij}$  may be MNAR, with  $f(\mathcal{R}_{ij} | Z_{i.}, \mathcal{R}_{i1}, \dots, \mathcal{R}_{i,j-1}) = f(\mathcal{R}_{ij} | Z_{ij}, W_{i.})$ .

In *Assumption 2*, we allow  $Z_{ij}$  to be MNAR such that its missingness depends on the true value of  $Z_{ij}$  but does not depend on other variables with missingness. We also assume that missingness is independent between variables assumed to be MNAR given  $Z$ .

### A.1 Imputation and weights under *Assumptions 1-2*

Imputation of  $Z_{i,d+1}, \dots, Z_{ik}$  will be the same as before, since these variables are assumed to be MAR and independent of missingness in the MNAR variables. Since we assume that missingness is independent between the MNAR variables and that missingness in each variable is independent of *other* variables with missingness, we can again re-write the imputation distribution for each MNAR variable  $Z_{ij}, j = 1, \dots, d$  as follows:

$$f(Z_{ij} | Z_{i,-j}, \mathcal{R}_{ij} = 0) \propto \frac{P(\mathcal{R}_{ij} = 0 | Z_{ij}, W_{i.})}{1 - P(\mathcal{R}_{ij} = 0 | Z_{ij}, W_{i.})} f(Z_{ij} | Z_{i,-j}, \mathcal{R}_{ij} = 1) \quad (\text{Eq. S1})$$

Suppose that instead of imputing from *Eq. S1* directly, we impute each  $Z_{ij}$  from  $f(Z_{ij} | Z_{i,-j}, \mathcal{R}_{ij} = 1)$ . We can collect the “weight” terms for each one of the imputed variables to obtain an aggregate weight to use for the final analysis as follows:

$$\omega_{im} \propto \prod_{j=1}^d \frac{P(\mathcal{R}_{ij} = 0 | Z_{ijm}, W_{i.})}{1 - P(\mathcal{R}_{ij} = 0 | Z_{ijm}, W_{i.})} \quad (\text{Eq. S2})$$

where  $Z_{ijm}$  is the  $m^{\text{th}}$  imputation of  $Z_{ij}$ . Suppose, now, that we can reasonably approximate each missingness model with a logistic regression model as follows:

$$\text{logit}(P(\mathcal{R}_{ij} = 1 | Z_{ij}, W_{i.})) = \phi_0 + \phi_j Z_{ij} + \phi_{Wj}^T W_{i.} \quad (\text{Eq. S3})$$

In this case, we can re-write the weight as

$$\omega_{im} \propto \prod_{j=1}^d \exp(-\phi_j Z_{ijm}) = \exp\left(-\sum_{j=1}^d \phi_j Z_{ijm}\right) \quad (\text{Eq. } S4)$$

This weight is a very simple function of the imputed data and  $d$  sensitivity parameters,  $\phi_1, \dots, \phi_d$ . Analysis can proceed as described in the main paper, where the form of the weights now depends on *multiple* sensitivity parameters, each describing the strength of the MNAR dependence of each variable and its own missingness. Although not shown in this paper, simulations demonstrate that this strategy can produce valid parameter estimates and corresponding standard errors as seen in the single-variable MNAR simulations presented here.

## A.2 Imputation and weights for more complicated MNAR mechanisms

Suppose we want to consider more general MNAR missingness. We now consider the form of the conditional distribution we want to impute from under a chained equations imputation philosophy:  $f(Z_{ij}|Z_{i,-j}, \mathcal{R}_i = R_i)$ . Recall,  $R_i$  is the data realization of random variable  $\mathcal{R}_i$  related to whether each of the variables is observed for subject  $i$ . We have that

$$\begin{aligned} f(Z_{ij}|Z_{i,-j}, \mathcal{R}_i = R_i) &= \frac{P(\mathcal{R}_i = R_i|Z_{i,-j})}{P(\mathcal{R}_i = R_i|Z_{i,-j})} f(Z_{ij}|Z_{i,-j}) \\ &= \frac{P(\mathcal{R}_i = R_i|Z_{i,-j})}{P(\mathcal{R}_i = R_i|Z_{i,-j})} \frac{P(\mathcal{R}_{ij} = 1|Z_{i,-j})}{P(\mathcal{R}_{ij} = 1|Z_{i,-j})} f(Z_{ij}|Z_{i,-j}, \mathcal{R}_{ij} = 1) \\ &\propto \frac{P(\mathcal{R}_i = R_i|Z_{i,-j})}{P(\mathcal{R}_{ij} = 1|Z_{i,-j})} f(Z_{ij}|Z_{i,-j}, \mathcal{R}_{ij} = 1) \end{aligned} \quad (\text{Eq. } S5)$$

This expression suggests that we might impute each  $Z_{ij}$  from  $f(Z_{ij}|Z_{i,-j}, \mathcal{R}_{ij} = 1)$  as discussed in the main paper and weight the multiple imputations proportional to the product of the remaining components of Eq. S5. After pulling the term constant in  $j$  out of the product, we can define weights as follows

$$\omega_{im} \propto \frac{P(\mathcal{R}_i = R_i|Z_{i,m})}{\prod_{j:\mathcal{R}_{ij}=0} P(\mathcal{R}_{ij} = 1|Z_{i,m})} \quad (\text{Eq. } S6)$$

where  $Z_{i,m}$  is the  $m^{\text{th}}$  imputation of  $Z_i$ . In general, this form of the weight could be complicated.

We consider the special case where  $\mathcal{R}_{ij} \perp \mathcal{R}_{ik}|Z_i$  for all  $k \neq j$ . Restated, assume that missingness for each variable is conditionally independent of the missingness of other variables, given the true values for  $Z_i$ . In this case, we can simplify

$$\omega_{im} \propto \left[ \prod_{j:\mathcal{R}_{ij}=1} P(\mathcal{R}_{ij} = 1|Z_{i,m}) \right] \times \left[ \prod_{j:\mathcal{R}_{ij}=0} \frac{P(\mathcal{R}_{ij} = 0|Z_{i,m})}{P(\mathcal{R}_{ij} = 1|Z_{i,m})} \right] \quad (\text{Eq. } S7)$$

Under logistic regression models for the missingness in each variable, the second product in Eq. S7 will have a simple, convenient form similar to Eq. S4, but the first product will not. In order to use the weight in Eq. S7, we will need to posit a model for each MNAR missingness mechanism. This may be complicated in general but could be a useful strategy for handling MNAR if the missingness model structure is well-understood.

We note that under *Assumptions 1-2* above,  $Z_{ij}$  is independent of missingness in *other* variables with missingness, so the term  $\prod_{j:\mathcal{R}_{ij}=1} P(\mathcal{R}_{ij} = 1|Z_{i,m})$  will be constant across variables in  $Z_{i,m}$  that are imputed. Under the same logic, the term  $\prod_{j:\mathcal{R}_{ij}=0} \frac{P(\mathcal{R}_{ij}=0|Z_{i,m})}{P(\mathcal{R}_{ij}=1|Z_{i,m})}$  could be rewritten as  $\prod_{j=1}^d \frac{P(\mathcal{R}_{ij}=0|Z_{i,m})}{P(\mathcal{R}_{ij}=1|Z_{i,m})}$ . When we rescale  $\omega_{im}$  such that  $\sum_{k=1}^M \omega_{ik} = 1$ , the first product term will drop out, and after we will end up with a weight as in Eq. S2.

## B Simulation 1: additional results for single variable missingness

**Figure B.1:** Distribution of linear regression  $Z_2$  coefficient for 100 imputed datasets under MAR assumptions. Points correspond to corresponding re-weighting of these estimates using the method in Carpenter et al. (2007) with *assumed* values of  $\phi_1$  in  $(-1.5, 1.5)$ . The true coefficient value for the regression for  $Z_2|Z_1$  is 0.50. The true missingness model log-odds ratio,  $\phi_1$ , is 1.

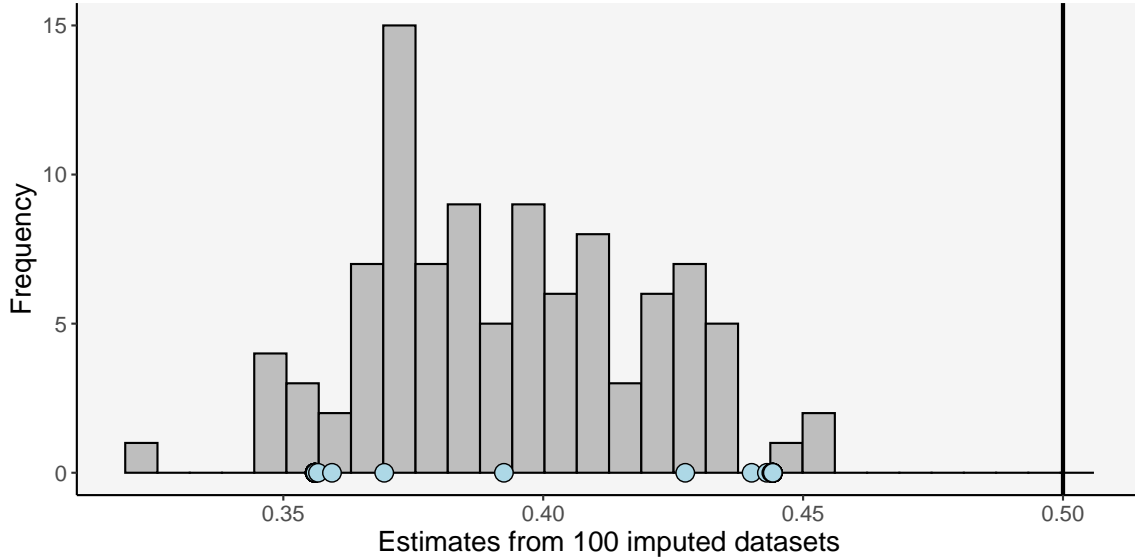

**Table B.1:** Bias in estimated  $Z_1|Z_2$  model parameters across 1000 simulated datasets for alternative MNAR-based chained equations methods and the proposed method ( $n=1000$ ,  $M=100$ ).  
1

| Method                 | $\phi_1$ | Intercept | Coefficient of $Z_2$ |
|------------------------|----------|-----------|----------------------|
| Truth                  | 1        | 0         | 0.5                  |
| Complete Case Analysis | 1        | 0.323     | 0.342                |
| Proposed Method        | 1        | -0.009    | 0.507                |
| Tompsett et al. (2018) | 1        | 0.003     | 0.500                |
| Jolani (2012)          | 1        | 0.411     | 0.297                |
| Truth                  | 0.5      | 0         | 0.5                  |
| Complete Case Analysis | 0.5      | 0.180     | 0.416                |
| Proposed Method        | 0.5      | -0.001    | 0.501                |
| Tompsett et al. (2018) | 0.5      | 0.005     | 0.498                |
| Jolani (2012)          | 0.5      | 0.266     | 0.376                |

<sup>1</sup>For the method in Tompsett et al. (2018), we did not adjust for missingness indicators for *other* variables when imputing  $Z_1$  and instead only incorporated the fixed offset as a function of  $R_{1.}$ . This method was implemented using the *mice.impute.mnar.norm* imputation method in R. The method in Jolani (2012) was implemented using *mice.impute.vi* imputation method in R. For the proposed method and the method in Tompsett et al. (2018), sensitivity parameters were fixed to the best possible value (which differs between the two methods).

**Figure B.2:** Weights assigned to each of 100 multiple imputations across different *assumed* values for  $\phi_1$  in  $(-1.5, 1.5)$  for normally-distributed  $Z_1$ . The true missingness model log-odds ratio,  $\phi_1$ , is 1.<sup>1</sup>

(a) Weights assigned to each of 100 imputed datasets (lines) for proposed method and Carpenter et al. (2007) method

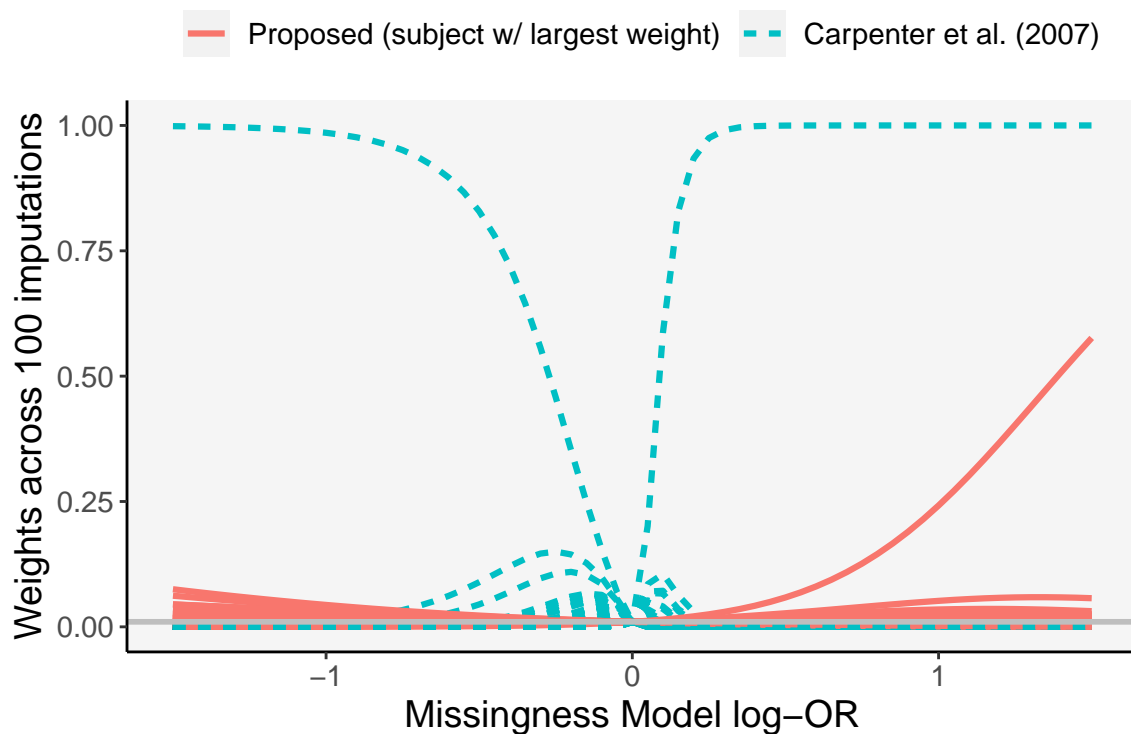

(b) Boxplots and densities of *proposed* weights across 100 multiple imputations for some example subjects

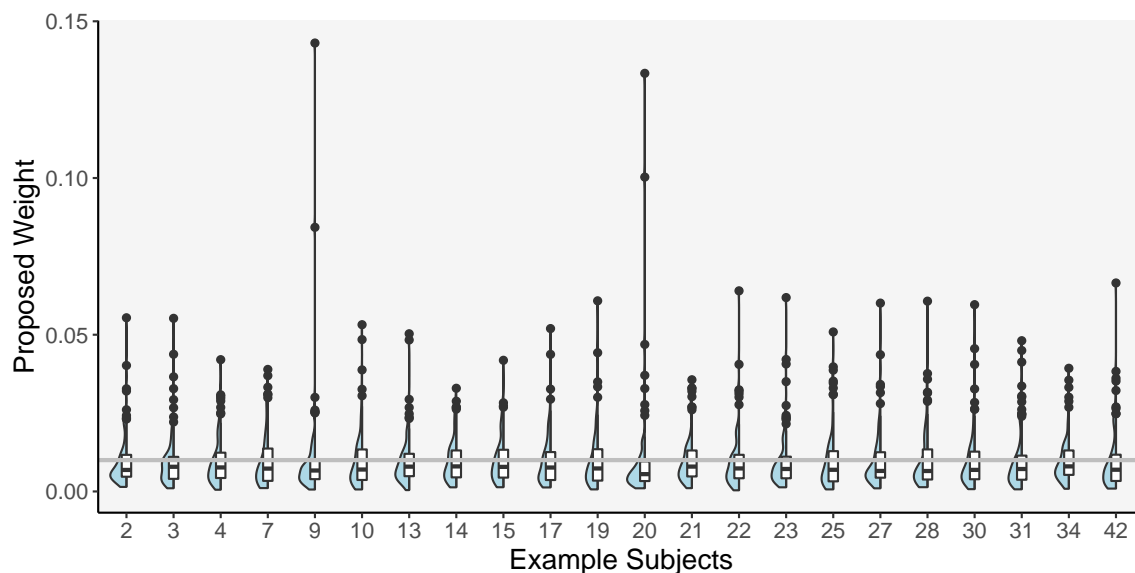

<sup>1</sup> For the method in Carpenter et al. (2007), weights are scaled to sum to 1 across imputed datasets. For the proposed methods, weights are scaled to sum to 1 across imputed datasets *within subjects*.

**Figure B.3:** Time to compute standard errors for linear regression based on stacked multiple imputations as a function of  $M$  ( $n = 1000$ )

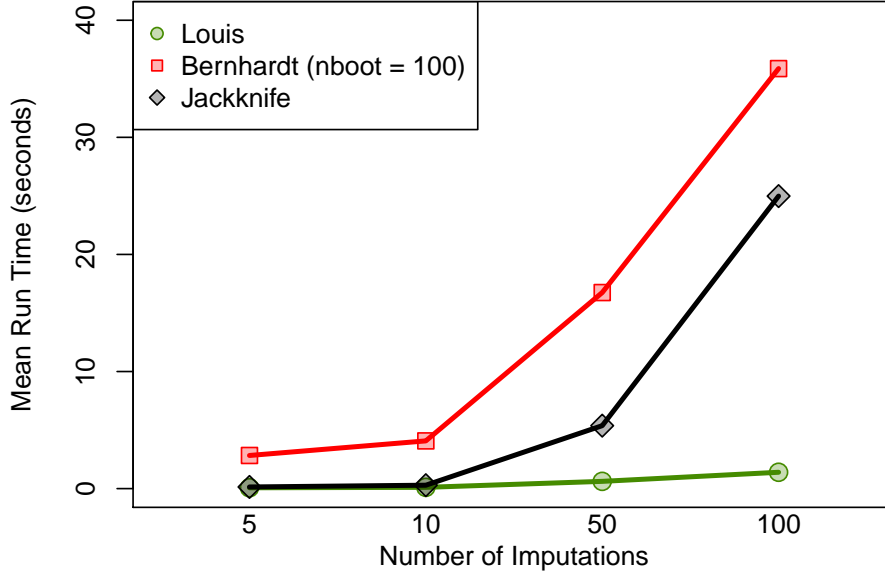

## C Simulation 2: missingness in multiple covariates

We now consider the case where we have missingness in multiple covariates. In each simulation setting, we generate 1000 simulated datasets of  $N = 2000$  subjects. In all settings, we generate covariates  $(Z_1, Z_2, Z_3)$  following a multivariate normal distribution with mean zero, standard deviation 1, and covariances of 0.3. We then generate  $Z_4$  under linear regression  $Z_4 \sim N(0 + 0.5Z_1 + 0.5Z_2 + 0.5Z_3, 1)$ . We impose MNAR missingness in  $Z_1$  under the following model:  $\text{logit}(P(R_1 = 1|Z)) = \phi_0 + \phi_1 Z_1 + 0.5Z_3 + 0.5Z_4$ . Missingness model parameters were specified to generate different degrees of deviation from MAR, with true missingness model log-odds ratio  $\phi_1$  taking values in -0.5, 0, 0.5, and 1.  $\phi_0$  was chosen to give roughly a 50% missingness rate for  $Z_1$ . We also generate 50% MCAR missingness in  $Z_2$ .

We then obtain 50 multiple imputations for missing values of  $Z_1$  and  $Z_2$  using the package *mice* in R assuming linear regression imputation models for each variable. Using these multiple imputations, we then estimate parameters in the model for  $Z_4|Z_1, Z_2, Z_3$  either using the method in Carpenter et al. (2007) or the proposed stacking and weighting method. Since  $\phi_1$  would be usually unknown in practice, we perform this estimation for different *assumed* values of log-odds ratio  $\phi_1$ .

**Figure C.1a** shows the bias in linear regression parameter estimates (model for  $Z_4|Z_1, Z_2, Z_3$ ) when  $\phi_1$  is *correctly specified*. As before, we find that our proposed approach can do a good job at estimating model parameters and that the method in Carpenter et al. (2007) can result in substantial residual bias. **Figure C.1b** provides the estimates across different *assumed* values for  $\phi_1$ , with the true value of  $\phi_1$  highlighted with a star.

**Figure C.1:** Average bias in estimated parameters from linear regression of  $Z_4|Z_1, Z_2, Z_3$  under MNAR missingness in covariate  $Z_1$  and MCAR missingness in covariate  $Z_2$ .

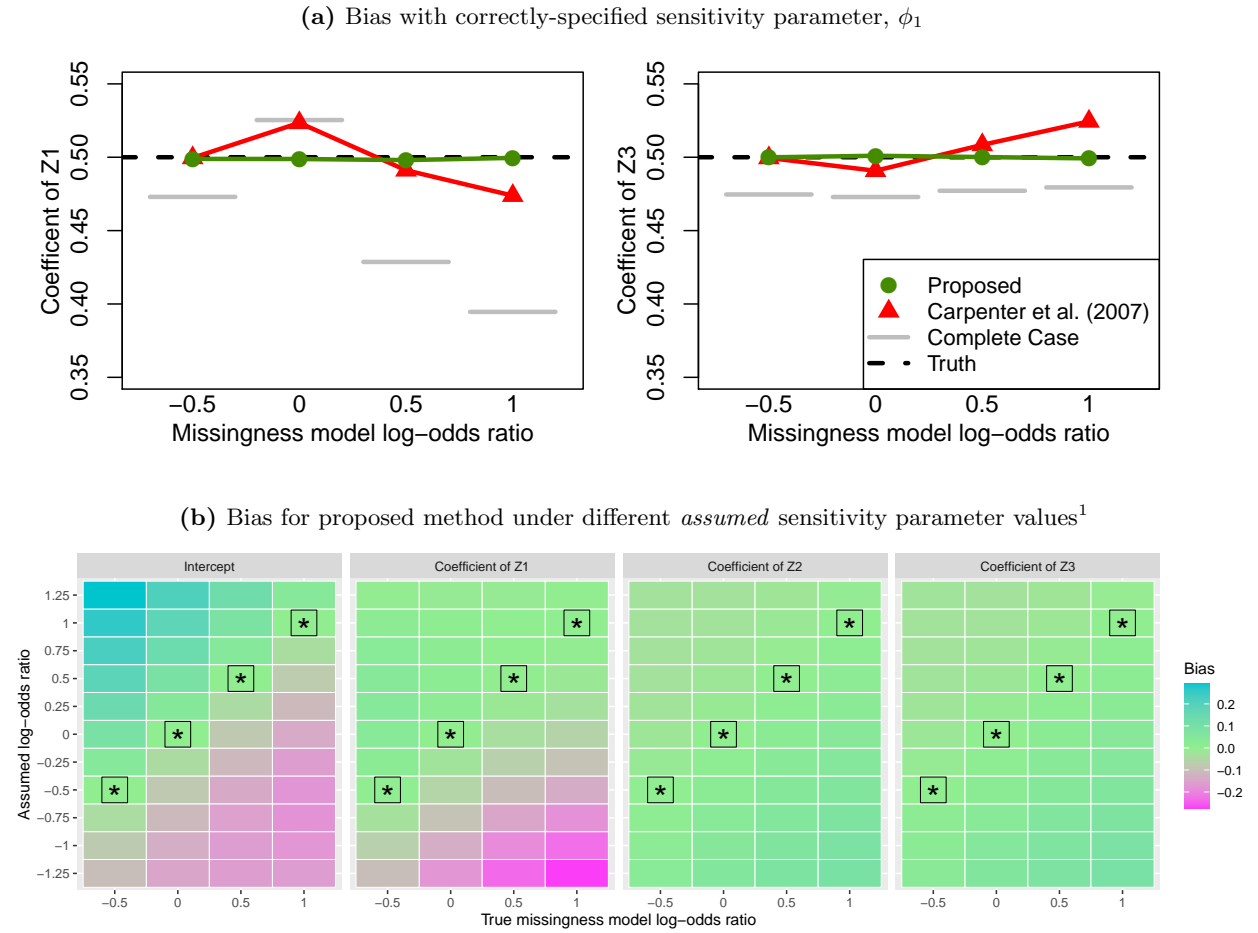

<sup>1</sup> The true value of  $\phi_1$  is highlighted for each simulation setting by ‘\*’.

An alternative imputation strategy is to apply the Tompsett et al. (2018) approach, where imputation of  $Z_{i1}$  uses  $1 - R_{i,-1}$  as a covariate and the coefficient for  $1 - R_{i,-1}$  is a fixed sensitivity parameter. Since we assume that  $Z_{i1}$  is independent of  $1 - R_{i,-1}$ , this approach reduces to performing imputation with a fixed offset proportional to  $(1 - R_{i,-1})$  with corresponding sensitivity parameter controlling the degree of deviation from MAR. This coefficient does not directly correspond to the coefficient in the missingness model. However, we can determine the best possible value of this offset parameter for our simulated data by fitting a regression model for true  $Z_{i1}$  given true  $Z_{i,-1}$  and  $R_{i1}$ . We use the resulting ideal parameter, which would not be known in real data analyses, to benchmark the performance of our proposed method relative to the strategy of including an offset in the imputation model. For  $\phi$  in -0.5, 0, 0.5, and 1, the ideal  $Z_{i1}$  model offset should be roughly 0.34, 0, -0.34, and -0.62, respectively.

**Figure C.2** provides bias in outcome model parameter estimates across different values of these alternative sensitivity parameters, where the ideal offset sensitivity parameter is shown for each of the 4 simulation settings along the x-axis. Generally, if we posit a values of the sensitivity parameter near the best possible value, this method can produce low bias. This simulation demonstrates that the Tompsett et al. (2018) approach can work in ideal settings, as can our method. The implementation is the primary difference here, where our sensitivity parameters correspond to the missingness model directly, and we only have to impute once rather than separately for each value of the sensitivity parameters.

**Figure C.2:** Average bias from fixed offset imputation method

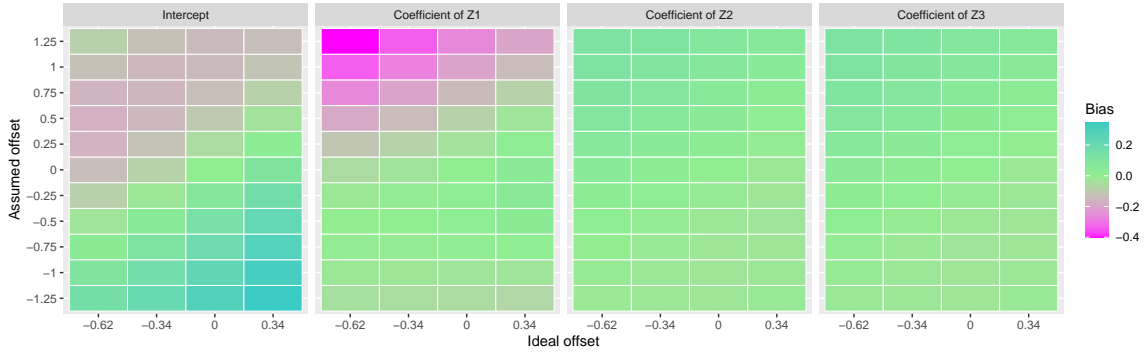

**Figure C.3** provides the average estimated variances and coverage of 95% confidence intervals for each of the three variance estimation strategies. We again find that the method in *Eq. 9* tends to produce slight under-coverage. Additionally, for large values of true  $\phi_1$ , the method from Bernhardt (2019) and our Jackknife modification both produce slight over-coverage. Coverage rates for logistic regression model parameters are near-nominal for all methods (not shown).

**Figure C.3:** Coverage of 95% confidence intervals and average estimated variances for linear regression coefficients from stacked and weighted analysis across 1000 simulated datasets, assuming true  $\phi_1$  is known

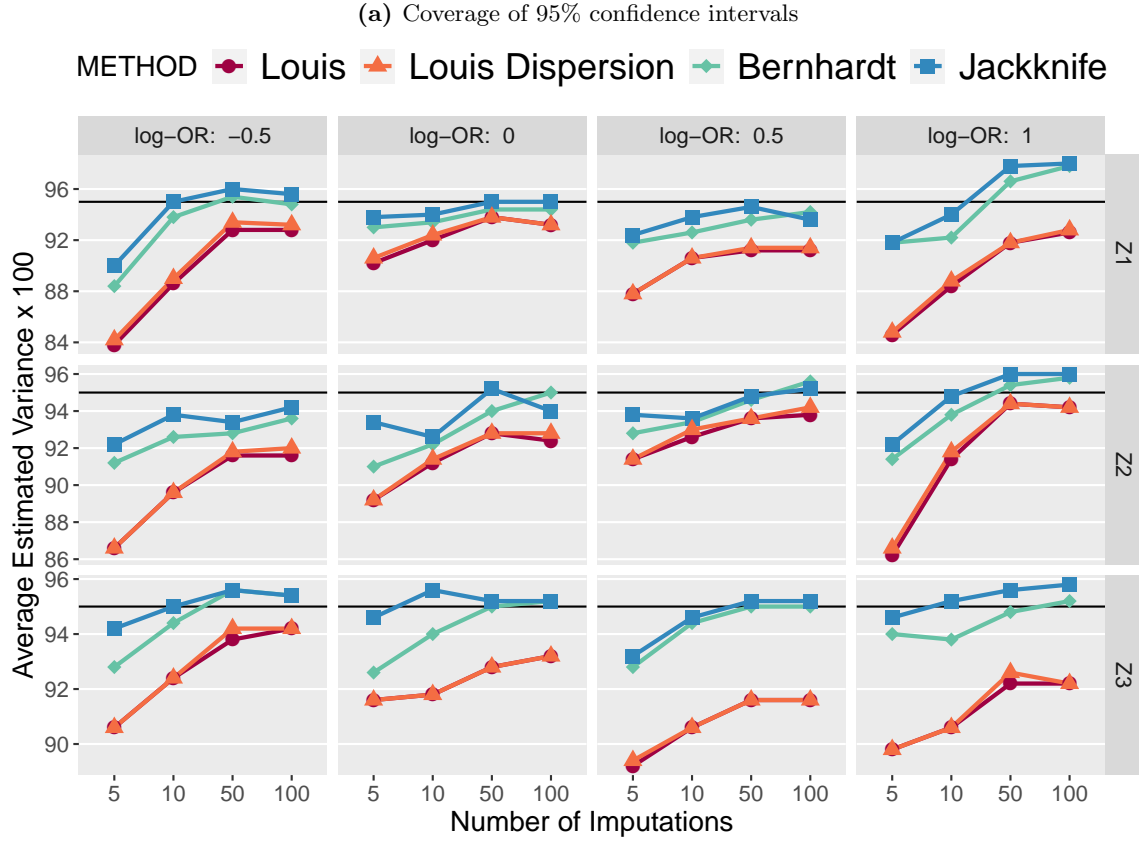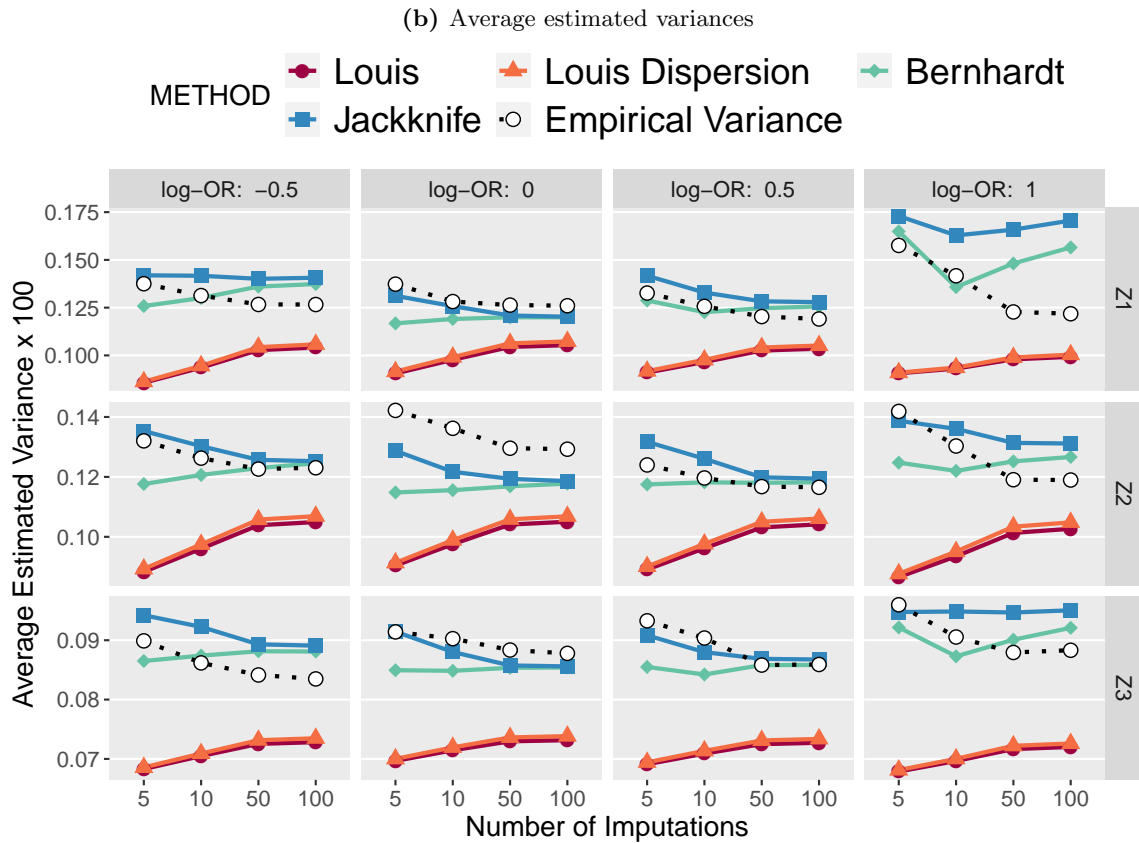

The “Louis Dispersion” method uses the estimator in Eq. 9 applied to imputed data obtained after fixing the imputation model dispersion parameters to the simulation truths.

**Table C.1:** Bias in estimated  $Z_4|Z_1, Z_2, Z_3$  model parameters across 1000 simulated datasets for alternative MNAR-based chained equations method and the proposed method (M=100). <sup>1</sup>

| Method                 | $\phi_1$ | Intercept | Coefficient of $Z_1$ | Coefficient of $Z_2$ | Coefficient of $Z_3$ |
|------------------------|----------|-----------|----------------------|----------------------|----------------------|
| Truth                  | 0        | 0         | 0.5                  | 0.5                  | 0.5                  |
| Complete Case Analysis | 0        | 0.236     | 0.473                | 0.375                | 0.475                |
| Proposed Method        | 0        | 0.000     | 0.499                | 0.499                | 0.500                |
| Tompsett et al. (2018) | 0        | 0.000     | 0.499                | 0.500                | 0.500                |
| Jolani (2012)          | 0        | -0.028    | 0.473                | 0.510                | 0.510                |
| Truth                  | -0.5     | 0         | 0.5                  | 0.5                  | 0.5                  |
| Complete Case Analysis | -0.5     | 0.234     | 0.525                | 0.472                | 0.473                |
| Proposed Method        | -0.5     | 0.000     | 0.499                | 0.498                | 0.501                |
| Tompsett et al. (2018) | -0.5     | 0.000     | 0.499                | 0.499                | 0.501                |
| Jolani (2012)          | -0.5     | 0.067     | 0.521                | 0.488                | 0.490                |
| Truth                  | 0.5      | 0         | 0.5                  | 0.5                  | 0.5                  |
| Complete Case Analysis | 0.5      | 0.236     | 0.429                | 0.477                | 0.477                |
| Proposed Method        | 0.5      | 0.001     | 0.498                | 0.500                | 0.500                |
| Tompsett et al. (2018) | 0.5      | 0.000     | 0.498                | 0.501                | 0.500                |
| Jolani (2012)          | 0.5      | -0.101    | 0.429                | 0.535                | 0.533                |
| Truth                  | 1        | 0         | 0.5                  | 0.5                  | 0.5                  |
| Complete Case Analysis | 1        | 0.235     | 0.395                | 0.482                | 0.479                |
| Proposed Method        | 1        | 0.002     | 0.500                | 0.500                | 0.499                |
| Tompsett et al. (2018) | 1        | 0.000     | 0.498                | 0.501                | 0.500                |
| Jolani (2012)          | 1        | -0.148    | 0.397                | 0.553                | 0.551                |

<sup>1</sup>For the method in Tompsett et al. (2018), we did not adjust for missingness indicators for *other* variables when imputing  $Z_{.1}$  and instead only incorporated the fixed offset as a function of  $R_{.1}$ . This method was implemented using the *mice.impute.mnar.norm* imputation method in R. The method in Jolani (2012) was implemented using *mice.impute.ri* imputation method in R. For the proposed method and the method in Tompsett et al. (2018), sensitivity parameters were fixed to the best possible value (which differs between the two methods).

## D Additional information for oropharynx cancer example

In this section, we provide some additional information about HPV missingness and the implementation of imputation assuming MAR. Missing values in HPV status (positive/negative), smoking status (current/former/never), T-stage (T1/T2/T3/T4), overall cancer stage (I/II/III/IV), and ACE7 comorbidities (none/mild/moderate/severe) were imputed 50 times using the method in White and Royston (2009) to generate the multiple imputations. These imputations are then stacked, and analysis proceeds using the proposed method.

For generating multiple imputations, we first obtained the Nelson-Aalen estimate for the cumulative hazard of all-cause survival, denoted  $\Lambda(T_i)$ , using the censored overall survival outcome and event indicator,  $\delta$ , in the data. Each covariate was then imputed using a regression model adjusting for other covariates along the  $\Lambda(T_i)$  and  $\delta$ . HPV status were imputed using a logistic regression model adjusting for gender, smoking status, age at diagnosis, overall cancer stage, ACE27 comorbidities, year of study enrollment,  $\Lambda(T_i)$  and  $\delta$ . Smoking status and ACE27 score were imputed using multinomial logistic regression adjusting for gender, HPV status, overall cancer stage, age at diagnosis,  $\Lambda(T_i)$ ,  $\delta$ , and either ACE27 score or smoking status, respectively. T-stage and overall cancer stage were both imputed using proportional odds regression adjusting for gender, smoking status, HPV status, comorbidities, age at diagnosis,  $\Lambda(T_i)$ ,  $\delta$ , and either overall cancer stage or T-stage, respectively.

**Figure D.1:** Observed and missing values of baseline HPV status by year of enrollment

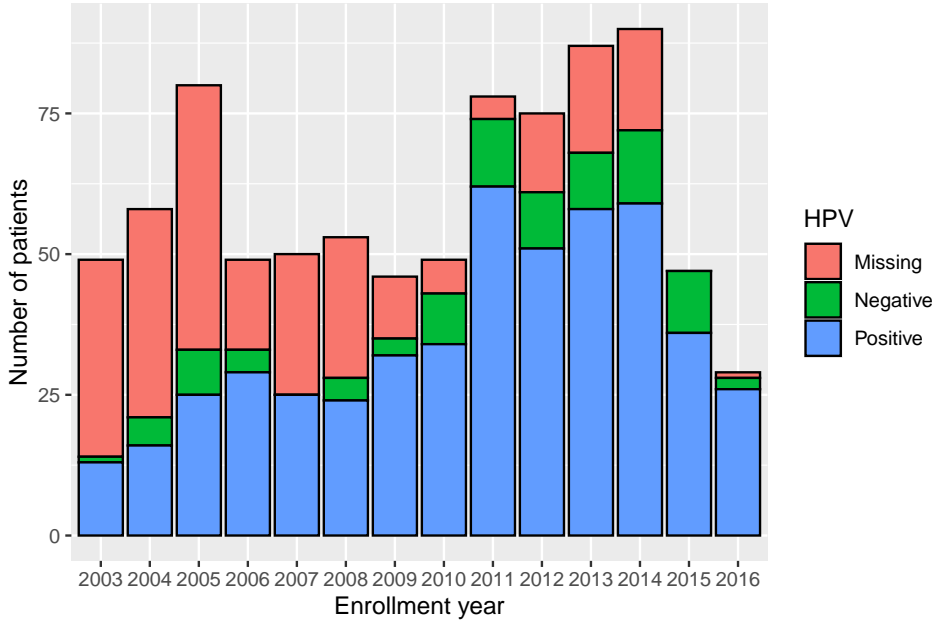

**Table D.1:** Logistic regression model estimates for the probability of observing HPV status <sup>1</sup>

| Characteristic                 | log-odds ratio (95% CI) |
|--------------------------------|-------------------------|
| Smoking                        |                         |
| Never                          | reference               |
| Former (> 12 months)           | -0.05 (-0.14, 0.03)     |
| Current (< 12 months)          | -0.13 (-0.21, -0.04)    |
| ACE27 comorbidities            |                         |
| None                           | reference               |
| Mild                           | 0.00 (-0.07, 0.09)      |
| Moderate                       | 0.04 (-0.07, 0.14)      |
| Severe                         | -0.17 (-0.32, -0.03)    |
| Age at diagnosis (decades)     | -0.04 (-0.08, 0.00)     |
| AJCC Cancer Stage              |                         |
| I                              | reference               |
| II                             | 0.04 (-0.30, 0.37)      |
| III                            | 0.03 (-0.27, 0.34)      |
| IV                             | 0.08 (-0.20, 0.37)      |
| Year of enrollment (2012-2016) | 0.06 (0.05, 0.07)       |

<sup>1</sup> among the  $N = 612$  subjects with fully-observed data for comorbidities, smoking status, and cancer stage.

## References

- Paul Bernhardt. A comparison of stacked and pooled multiple imputation. In *Joint Statistical Meetings Poster Presentation*, 2019.
- James R Carpenter, Michael G Kenward, and Ian R White. Sensitivity analysis after multiple imputation under missing at random: a weighting approach. *Statistical Methods in Medical Research*, 16(3):259–275, 2007.
- Shahab Jolani. *Dual Imputation Strategies for Analyzing Incomplete Data*. PhD thesis, Utrecht University, 2012.
- Daniel Mark Tompsett, Finbarr Leacy, Margarita Moreno-Betancur, Jon Heron, and Ian R White. On the use of the not-at-random fully conditional specification (NARFCS) procedure in practice. *Statistics in Medicine*, 37(15):2338–2353, 2018. doi: 10.1002/sim.7643.
- Ian R White and Patrick Royston. Imputing missing covariate values for the Cox model. *Statistics in Medicine*, 28(15):1982–1998, 2009.
